# Supplementary material for: A Preconditioned Semismooth Newton Method for Box-Constrained Elliptic Optimal Control Problems with Random Coefficients
Source: arXiv:2611.00246 source file (2026-10-30)
Supplement: Supplementary file 1 [file appendix.tex]

% Appendix A of ex_article.tex (to be input right after \appendix).
% It compares the scalar free-fraction preconditioner P_vartheta, that is,
% the preconditioner P_k of Section 6, with the current-set
% preconditioner P_W of Section 5.2.

\section{The scalar free-fraction preconditioner
\texorpdfstring{$P_\vartheta$}{P\_theta}}\label{app:wm-scalar}
The spectral enclosures of Section~\ref{sec:ssn} concern the current-set
preconditioner $P_W=H_0+\gamma^{-1}C_D$ of \eqref{eq:wm-JP}, which contains
the active-set term $\gamma^{-1}C_D$ exactly and is applied through the formula of Proposition~\ref{prop:wm-woodbury}.  The experiments of
Section~\ref{sec:numerics} use instead the cheaper preconditioner $P_k$,
which keeps only the stored free fraction
$\widehat\vartheta_k=\operatorname{Tr}D(p_j)/m$ of the most recent
refactorization step $j\le k$ and ignores where the free set lies.  This
appendix compares
the scalar family $P_\vartheta$, $\vartheta\ge0$, of \eqref{eq:wm-Ptheta},
which contains $P_k=P_{\widehat\vartheta_k}$, with $P_W$.
Theorem~\ref{thm:wm-equiv} shows that, for every
$\vartheta\ge0$, the eigenvalues of $P_\vartheta^{-1}P_W$ lie in an
explicit interval.  Under Assumption~\ref{ass:wm-local}, this interval is
independent of $h$, of $n_\xi$ and of the mask, including the location of
its free set.
The regularization parameter $\gamma$ enters this interval only through the
number $\varepsilon_\gamma$ of \eqref{eq:wm-epsgamma}, which is proportional
to $\gamma^{-1}$.  Theorem~\ref{thm:wm-count}
counts the eigenvalues outside $[\tau,1]$ for a threshold $0<\tau<1$.
% Part~(c) shows that, on a model problem, this dependence on $\gamma$ cannot
% be removed by any choice of $\vartheta$, nor by any other preconditioner
% that takes the same value at two masks that are mirror images of each
% other.

A symmetric matrix $A$ is positive semidefinite, written $A\succeq0$, if
$v^\top Av\ge0$ for all $v$, and symmetric positive definite (SPD), written
$A\succ0$, if $v^\top Av>0$ for all $v\ne0$.  For symmetric $A$ and $B$ of
equal size, $A\preceq B$ means $B-A\succeq0$ (the Loewner order).  For a
diagonal matrix $D$, the inequalities $0\le D\le I$ are understood entrywise.
For $A=A^\top$ and $B\succ0$ in $\R^{n\times n}$, we denote by
$\lambda_1(A,B)\le\dots\le\lambda_n(A,B)$ the eigenvalues of $B^{-1}A$, repeated according to multiplicity.  They are
real by Lemma~\ref{lem:wm-pencil}(a).  We denote by $n_{>t}(A,B)$ and
$n_{<t}(A,B)$ the numbers of them that are larger, respectively smaller,
than $t\in\R$.  For a symmetric matrix $X$, $\iota_+(X)$ and $\iota_-(X)$
denote the numbers of positive and negative eigenvalues of $X$, counted
with multiplicity.  For SPD matrices $A$ and $B$ of equal size, the
eigenvalues of $A^{-1}B$ are real and positive, and define
\[
\kappa_{\rm sp}(A^{-1}B) \coloneqq \frac{\lambda_{\max}(A^{-1}B)}{\lambda_{\min}(A^{-1}B)}.
\]
It is
the condition number of the SPD matrix $A^{-1/2}BA^{-1/2}$.  For
$A=P_\vartheta$ and $B=J$, it is the quantity that governs the PCG bound
\eqref{eq:wm-pcg} when $P_\vartheta$ replaces $P_W$.

We use the notation of Section~\ref{sec:woodbury}, with $n_\xi=N_P$ and
$N=n_\xi n_h$: $\mathcal M=I_{n_\xi}\otimes M_D$,
$\overline{\mathcal K}=I_{n_\xi}\otimes K_0$ and $\mathcal K$ are the
matrices of \eqref{eq:wm-SG}, and, as in \eqref{eq:wm-JP},
\begin{gather*}
 H=\mathcal K\mathcal M^{-1}\mathcal K^\top,\qquad
 H_0=\overline{\mathcal K}\mathcal M^{-1}\overline{\mathcal K}^\top
 =I_{n_\xi}\otimes K_0M_D^{-1}K_0,\\
 J=H+\gamma^{-1}C_D,\qquad P_W=H_0+\gamma^{-1}C_D,
\end{gather*}
where the symmetry of $K_0$ was used.
As in Section~\ref{sec:sgfe}, the
control values are indexed by pairs $(k,r)$, where $\xi_k$ ($1\le k\le n_q$)
is a stochastic quadrature point and $x_r$ ($1\le r\le n_h$) is an interior
node with $r$ running fastest. Thus $m\coloneqq n_qn_h$ is the number of control
values, $E=V_\xi\otimes I_{n_h}\in\R^{m\times N}$ and
$W=W_\xi\otimes M_L\in\R^{m\times m}$.
The active-set term is $\gamma^{-1}C_D$, where
\[
 C_D=E^\top WDE,\qquad D=\operatorname{diag}(D_{(k,r)})\in\R^{m\times m},
 \qquad 0\le D\le I_m .
\]
The algorithm uses the binary mask $D=D(p)$ of Section~\ref{sec:ssn}.
% The analysis also admits fractional values.
We use $P_W(D)$ and~$J(D)$ when
the dependence on the mask matters.
The constants
$c$ and $C$ of Theorem~\ref{thm:wm-algebra} are called $c_H$ and $C_H$
here, to distinguish them from $c_\vartheta$.  The bound
$c_HH_0\preceq H\preceq C_HH_0$ holds at a fixed discretization with
$c_H=s_-^2$ and $C_H=s_+^2$ by Lemma~\ref{lem:wm-reduction}.  Under the
hypotheses of Corollary~\ref{cor:wm-uniform}, it holds with
$c_H=V^{-2}$ and $C_H=U^2$, independent of $h$, $n_\xi$ and $s$.
The free fraction $\vartheta$ is unrelated to the constants
$\theta_\pm$ of Theorem~\ref{thm:wm-algebra} and to the angles $\theta_r$
in the proof of Lemma~\ref{lem:wm-reference}.

We assume that the stochastic quadrature rule integrates every product
$\psi_i\psi_j$ exactly, i.e.,
\begin{equation}\label{eq:wm-exactquad}
  V_\xi^{\top} W_\xi V_\xi = I_{n_\xi}.
\end{equation}
This holds, for instance, for a total-degree polynomial basis of degree $P$
combined with the tensor-product Gauss--Legendre rule with $P+1$ points per
direction.

% \emph{The scalar preconditioner.}
For $0\le\vartheta\le1$, the uniform mask $D=\vartheta I_m$ has the
active-set term
$\gamma^{-1}C_{\vartheta I_m}=(\vartheta/\gamma)I_{n_\xi}\otimes M_L$ by
Lemma~\ref{lem:wm-lump}(c), and replacing the lumped mass $M_L$ by the
consistent mass $M_D$ turns this term into $(\vartheta/\gamma)\mathcal M$.
For $\vartheta\ge0$ put
$c_\vartheta \coloneqq (\vartheta/\gamma)^{1/2}$ and
\begin{equation}\label{eq:wm-Ptheta}
 \begin{aligned}
 P_\vartheta& \coloneqq (\overline{\mathcal K}+c_\vartheta\mathcal M)\mathcal M^{-1}
   (\overline{\mathcal K}+c_\vartheta\mathcal M)
   =H_0+2c_\vartheta\overline{\mathcal K}+c_\vartheta^2\mathcal M\\
 &\hphantom{:}=I_{n_\xi}\otimes\bigl[(K_0+c_\vartheta M_D)M_D^{-1}
   (K_0+c_\vartheta M_D)\bigr],
 \end{aligned}
\end{equation}
where $\overline{\mathcal K}=\overline{\mathcal K}^\top$ was used.
% Thus $P_0=H_0$, $P_1$ is the matching preconditioner $P_{\rm mean}$ of Section~\ref{sec:numerics}, and the preconditioner used there is
% $P_k=P_{\widehat\vartheta_k}$, with $c_k=c_{\widehat\vartheta_k}$ and
% $S_k=K_0+c_kM_D$.  Compared with $P_W$, the matrix $P_\vartheta$ replaces
% the active-set term $\gamma^{-1}C_D$ by $(\vartheta/\gamma)\mathcal M$ and
% adds the cross term $2c_\vartheta\overline{\mathcal K}$ of the matching factorization.
% Only the scalar $\vartheta$ enters $P_\vartheta$, not the location of the free set.

Let $\Lambda_L\ge1$ and $\underline\lambda>0$
satisfy
\begin{equation}\label{eq:wm-lump}
 M_D\preceq M_L\preceq\Lambda_LM_D,\qquad K_0\succeq\underline\lambda\,M_D .
\end{equation}
% The first condition compares the lumped mass
% $M_L=\operatorname{diag}(M_D\bm 1)$, which enters the control weights $W$
% with the consistent mass $M_D$, which enters $\mathcal M$; the second one
% is a lower bound for the spectrum of $M_D^{-1}K_0$.
The first condition relates the lumped mass
$M_L=\operatorname{diag}(M_D\bm{1})$, which determines the control weights $W$,
to the consistent mass $M_D$, which enters $\mathcal{M}$. And the second imposes a
lower bound on the spectrum of $M_D^{-1}K_0$.
Let
$0<\lambda^h_1\le\dots\le\lambda^h_{n_h}$ be the eigenvalues of
$M_D^{-1}K_0$, repeated according to multiplicity, and let
\[
 \mathcal N_h(\lambda) \coloneqq \#\{j:\lambda^h_j<\lambda\},\qquad\lambda\ge0,
\]
be their counting function. The largest admissible $\underline\lambda$ in
\eqref{eq:wm-lump} is $\lambda^h_1$.  Since $\lambda^h_1$ depends on $h$,
bounds uniform in $h$ need $h$-independent values.  Under
Assumption~\ref{ass:wm-local}, Lemma~\ref{lem:wm-lump}(b) gives
$\Lambda_L=9$ and $\underline\lambda=\lambda_*=8\nu_-/d^2$, and
Lemma~\ref{lem:wm-weyl}(a) gives the larger, hence sharper, value
$\underline\lambda=2\pi^2\nu_-/d^2$.

% {The parameters $\varepsilon_\gamma$, $\varsigma_\vartheta$ and
% $\chi_\gamma$.}
Define
\begin{equation}\label{eq:wm-epsgamma}
 \varepsilon_\gamma \coloneqq \frac{1}{\gamma\underline\lambda^{2}},\qquad
 \varsigma_\vartheta \coloneqq \frac{c_\vartheta}{\underline\lambda}
   =(\vartheta\varepsilon_\gamma)^{1/2},\qquad
 \chi_\gamma(\vartheta) \coloneqq \max\bigl\{(1+\varsigma_\vartheta)^2,\,
   1+\Lambda_L\varepsilon_\gamma\bigr\}.
\end{equation}
The number $\varepsilon_\gamma$ compares the active-set term with $H_0$ on
the smoothest spatial mode.  Indeed, $H_0\succeq\underline\lambda^2\mathcal M$
by Lemma~\ref{lem:wm-modal}, with equality on the modes of $\lambda^h_1$ if
$\underline\lambda=\lambda^h_1$.  By Lemma~\ref{lem:wm-lump}(c),
$0\preceq\gamma^{-1}C_D\preceq\Lambda_L\gamma^{-1}\mathcal M$, and hence, by the
preceding inequality, $0\preceq\gamma^{-1}C_D\preceq\Lambda_L\varepsilon_\gamma H_0$.  Thus $P_W$
is a small perturbation of $H_0=P_0$ when $\varepsilon_\gamma\ll1$.  For
$\varepsilon_\gamma\gg1$, the active-set term dominates on the smooth
modes for some masks.  For instance, for $D=I_m$,
$\gamma^{-1}C_D=\gamma^{-1}I_{n_\xi}\otimes M_L\succeq\gamma^{-1}\mathcal M$
by Lemma~\ref{lem:wm-lump}(c) and \eqref{eq:wm-lump}, and
$\gamma^{-1}\mathcal M$ equals $\varepsilon_\gamma H_0$ on the modes of
$\lambda^h_1$ if $\underline\lambda=\lambda^h_1$.  Likewise,
$\varsigma_\vartheta$ measures the correction
$P_\vartheta-H_0=2c_\vartheta\overline{\mathcal K}+c_\vartheta^2\mathcal M$.
On the $j$th spatial mode, $P_\vartheta$ exceeds $H_0$ by the factor
$(1+c_\vartheta/\lambda^h_j)^2\le(1+\varsigma_\vartheta)^2$.  Finally,
$\chi_\gamma(\vartheta)$ is the resulting bound for
$\kappa_{\rm sp}(P_\vartheta^{-1}P_W)$ in Theorem~\ref{thm:wm-equiv}(b).
% For example, with $\underline\lambda=2\pi^2\nu_-/d^2$
% (Lemma~\ref{lem:wm-weyl}(a)), Example~2 of Section~\ref{sec:numerics}
% ($d=2$, mean coefficient $1$) has $\underline\lambda=\pi^2/2$ and
% $\varepsilon_\gamma\approx0.0411/\gamma$, so that
% $\varepsilon_\gamma\approx41$ for $\gamma=10^{-3}$; Example~1 (mean
% coefficient $10$) has $\varepsilon_\gamma\approx4.11\times10^{-4}/\gamma$,
% that is, $\varepsilon_\gamma\approx0.41$ for $\gamma=10^{-3}$.

The first two theorems below rest on one structural fact.  The matrices
$\mathcal M$, $H_0$ and $P_\vartheta$ are diagonalized simultaneously by the
spatial modes, the eigenvectors of $M_D^{-1}K_0$
(Lemma~\ref{lem:wm-modal}).  Since $0\preceq C_D\preceq\Lambda_L\mathcal M$
(Lemma~\ref{lem:wm-lump}), $P_W$ lies between $H_0$ and
$H_0+\Lambda_L\gamma^{-1}\mathcal M$, and both bounds are diagonal in the
modal basis.  On each mode, the comparison with $P_\vartheta$ thus becomes a
scalar inequality between $(\lambda^h_j)^2$,
$(\lambda^h_j)^2+\Lambda_L\gamma^{-1}$ and $(\lambda^h_j+c_\vartheta)^2$
(Lemma~\ref{lem:wm-scalarfn}).  This gives Theorem~\ref{thm:wm-equiv}.
For Theorem~\ref{thm:wm-count}, the eigenvalues of $P_\vartheta^{-1}H_0$
are explicit.  Sylvester's law of inertia shows that adding
$\gamma^{-1}C_D$ changes the number of them on either side of a threshold
by at most $\operatorname{rank}C_D$ (Lemma~\ref{lem:wm-inertia}).  The
number of small ones is bounded independently of $h$ because, on the
uniform $Q_1$ mesh, the discrete Dirichlet eigenvalues lie above the
continuous ones (Lemmas~\ref{lem:wm-theta} and~\ref{lem:wm-weyl}).  For
Theorem~\ref{thm:wm-obstr}, test vectors supported on one half of a square
show that the current-set preconditioners of two mirror masks are far
apart in Hilbert's projective metric
(Lemmas~\ref{lem:wm-mirror}--\ref{lem:wm-rho}).  The triangle inequality
for this metric (Lemma~\ref{lem:wm-hilbert}) then shows that no single SPD
matrix is close to both.

The proof of Theorem~\ref{thm:wm-equiv} compares the eigenvalues of matrices $B^{-1}A$ through
Rayleigh quotients and congruences, which the next lemma collects.

\begin{lemma}[Rayleigh quotients and congruence]\label{lem:wm-pencil}
Let $A=A^\top$ and $B\succ0$ in $\R^{n\times n}$, and let $X$ and $X'$ be
symmetric $n\times n$ matrices.
\begin{enumerate}[label=\textup{(\alph*)},leftmargin=*]
\item The matrix $B^{-1}A$ is diagonalizable with real eigenvalues, and
 for $t_-\le t_+$ one has $\operatorname{spec}(B^{-1}A)\subset[t_-,t_+]$
 if and only if $t_-B\preceq A\preceq t_+B$.  The extreme eigenvalues are
 the extreme Rayleigh quotients:
 \[
  \lambda_1(A,B)=\min_{v\ne0}\frac{v^\top Av}{v^\top Bv},\qquad
  \lambda_n(A,B)=\max_{v\ne0}\frac{v^\top Av}{v^\top Bv}.
 \]
\item For invertible $G$, the matrices $B^{-1}A$ and $(G^\top BG)^{-1}G^\top AG$
 have the same eigenvalues with multiplicities, and for $p\ge1$ the matrix
 $(I_p\otimes B)^{-1}(I_p\otimes A)$ has the eigenvalues of $B^{-1}A$, each
 repeated $p$ times.  If $X\preceq X'$, then
 $I_p\otimes X\preceq I_p\otimes X'$.
\end{enumerate}
\end{lemma}

\begin{proof}
(a) Let $B=LL^\top$ be the Cholesky factorization and
$C \coloneqq L^{-1}AL^{-\top}$.  Then $B^{-1}A=L^{-\top}CL^\top$ is similar to the
symmetric matrix $C$.  Hence it is diagonalizable with the real eigenvalues
of $C$.  Congruence with $L^{-1}$ shows that $t_-B\preceq A\preceq t_+B$ is
equivalent to $t_-I\preceq C\preceq t_+I$, that is, to
$\operatorname{spec}(C)\subset[t_-,t_+]$.  With $w=L^\top v$, the Rayleigh
quotients $v^\top Av/v^\top Bv$ of $(A,B)$ are the Rayleigh quotients
$w^\top Cw/w^\top w$ of $C$, which gives the formulas for $\lambda_1(A,B)$
and $\lambda_n(A,B)$.

(b) The first two statements follow from
$(G^\top BG)^{-1}G^\top AG=G^{-1}(B^{-1}A)G$ and
$(I_p\otimes B)^{-1}(I_p\otimes A)=I_p\otimes B^{-1}A$.  The last one holds
because $I_p\otimes(X'-X)$ is block diagonal with diagonal blocks
$X'-X\succeq0$.
\end{proof}

The next lemma bounds the active-set term $\gamma^{-1}C_D$ by
$\Lambda_L\gamma^{-1}\mathcal M$, which gives the upper end
$H_0+\Lambda_L\gamma^{-1}\mathcal M$ of the enclosure of $P_W$.

\begin{lemma}[Lumped mass and the active-set term]\label{lem:wm-lump}
\begin{enumerate}[label=\textup{(\alph*)},leftmargin=*]
\item If $M_D$ is symmetric with nonnegative entries, then for every
 $g\in\R^{n_h}$
 \[
  g^\top(M_L-M_D)g=\frac12\sum_{r,s=1}^{n_h}(M_D)_{rs}(g_r-g_s)^2\ge0.
 \]
 Thus $M_D\preceq M_L$.
\item Under Assumption~\ref{ass:wm-local}, $M_D$ has nonnegative entries
 and $M_L\preceq h^2I\preceq9M_D$.  Hence \eqref{eq:wm-lump} holds with
 $\Lambda_L=9$, and with $\underline\lambda=\lambda_*$ by
 Lemma~\ref{lem:wm-reference}.
\item Assume \eqref{eq:wm-exactquad}.  Then $E^\top WE=I_{n_\xi}\otimes M_L$,
 and for every diagonal $0\le D\le I_m$
 \[
  0\preceq C_D\preceq I_{n_\xi}\otimes M_L .
 \]
 If $M_L\preceq\Lambda_LM_D$, then
 $I_{n_\xi}\otimes M_L\preceq\Lambda_L\mathcal M$, and hence
 $0\preceq C_D\preceq\Lambda_L\mathcal M$.
\end{enumerate}
\end{lemma}

\begin{proof}
(a) Since $M_L$ is diagonal with entries $(M_L)_{rr}=\sum_s(M_D)_{rs}$,
\[
 g^\top(M_L-M_D)g=\sum_{r,s}(M_D)_{rs}(g_r^2-g_rg_s).
\]
Interchanging $r$ and $s$ and using the symmetry of $M_D$, the right-hand
side also equals $\sum_{r,s}(M_D)_{rs}(g_s^2-g_rg_s)$.  The average of the
two expressions is the asserted identity.

(b) The bilinear nodal functions $\phi_r$ are products of one-dimensional
hat functions, so $\phi_r\ge0$.  Since the mass is integrated exactly,
$(M_D)_{rs}=\int\phi_r\phi_s\,dx\ge0$.  The nodal functions of all nodes,
including the eliminated boundary nodes, are nonnegative and sum to one.
Hence, for an interior node $x_r$,
\[
 (M_L)_{rr}=\int\phi_r\sum_{s\ \text{interior}}\phi_s\,dx
 \le\int\phi_r\,dx=h^2,
\]
because $\phi_r$ is supported on four elements and has integral $h^2/4$ on
each of them.  Thus $M_L\preceq h^2I$, and $h^2I\preceq9M_D$ is the first
inequality in \eqref{eq:wm-referencebounds}.  Together with (a) this gives
$M_D\preceq M_L\preceq9M_D$, and $K_0\succeq\lambda_*M_D$ is the last
inequality in \eqref{eq:wm-referencebounds}.

(c) By the mixed-product rule and \eqref{eq:wm-exactquad},
$E^\top WE=(V_\xi^\top W_\xi V_\xi)\otimes M_L=I_{n_\xi}\otimes M_L$.  The
matrices $W$ and $D$ are diagonal, $W$ has positive entries and
$0\le D\le I_m$.  Hence, for $v\in\R^N$ and $y \coloneqq Ev$,
\[
 0\le v^\top C_Dv=\sum_qW_{qq}D_{qq}y_q^2\le\sum_qW_{qq}y_q^2
 =v^\top E^\top WEv .
\]
Finally, $M_L\preceq\Lambda_LM_D$ and Lemma~\ref{lem:wm-pencil}(b) give
$I_{n_\xi}\otimes M_L\preceq\Lambda_LI_{n_\xi}\otimes M_D=\Lambda_L\mathcal M$.
\end{proof}

The next lemma diagonalizes $\mathcal M$, $H_0$ and $P_\vartheta$
simultaneously by the spatial modes.  Its part~(b) is used for
Theorem~\ref{thm:wm-count}.

\begin{lemma}[Modal form]\label{lem:wm-modal}
Let $\vartheta\ge0$, let $X_h\in\R^{n_h\times n_h}$ satisfy
\[
 X_h^\top M_DX_h=I,\qquad
 X_h^\top K_0X_h=\Lambda_h \coloneqq \operatorname{diag}(\lambda^h_1,\dots,\lambda^h_{n_h}),
\]
and put $\widetilde X_h \coloneqq I_{n_\xi}\otimes X_h$.  Then
\[
 \widetilde X_h^\top\mathcal M\widetilde X_h=I,\qquad
 \widetilde X_h^\top H_0\widetilde X_h=I_{n_\xi}\otimes\Lambda_h^2,\qquad
 \widetilde X_h^\top P_\vartheta\widetilde X_h
 =I_{n_\xi}\otimes(\Lambda_h+c_\vartheta I)^2 .
\]
\begin{enumerate}[label=\textup{(\alph*)},leftmargin=*]
\item The eigenvalues of $P_\vartheta^{-1}H_0$ are the numbers
 $(\lambda^h_j/(\lambda^h_j+c_\vartheta))^2$, $j=1,\dots,n_h$, each
 repeated $n_\xi$ times.
\item Let $0<\tau<1$ and
 $\lambda_\tau \coloneqq c_\vartheta\sqrt\tau/(1-\sqrt\tau)$.  For
 $\lambda>0$, $\lambda^2/(\lambda+c_\vartheta)^2<\tau$ exactly when
 $\lambda<\lambda_\tau$, and exactly $n_\xi\mathcal N_h(\lambda_\tau)$
 of the eigenvalues in \textup{(a)} are smaller than $\tau$.
\item One has
 $H_0\succeq(1+c_\vartheta/\lambda^h_1)^{-2}P_\vartheta$.  If
 $K_0\succeq\underline\lambda M_D$, then
 $H_0\succeq(1+\varsigma_\vartheta)^{-2}P_\vartheta$.
\end{enumerate}
\end{lemma}

\begin{proof}
The matrix $X_h$ exists because $K_0$ and $M_D$ are SPD.  From
$X_h^\top M_DX_h=I$ we get $M_D^{-1}=X_hX_h^\top$.  Hence, for $c\ge0$,
\[
 X_h^\top(K_0+cM_D)M_D^{-1}(K_0+cM_D)X_h
 =\bigl[X_h^\top(K_0+cM_D)X_h\bigr]^2=(\Lambda_h+cI)^2 .
\]
With $c=0$ and $c=c_\vartheta$, the identities $\mathcal M=I_{n_\xi}\otimes
M_D$ and $H_0=I_{n_\xi}\otimes K_0M_D^{-1}K_0$ and \eqref{eq:wm-Ptheta}
give the three congruences.

(a) By Lemma~\ref{lem:wm-pencil}(b), the matrix $P_\vartheta^{-1}H_0$ has
the eigenvalues of the diagonal matrix
$I_{n_\xi}\otimes\Lambda_h^2(\Lambda_h+c_\vartheta I)^{-2}$,
which are the numbers $(\lambda^h_j/(\lambda^h_j+c_\vartheta))^2$, each
repeated $n_\xi$ times.

(b) For $\lambda>0$ and $c\ge0$, $\lambda^2/(\lambda+c)^2<\tau$ holds if and
only if $\lambda<\sqrt\tau(\lambda+c)$, that is, if and only if
$\lambda<c\sqrt\tau/(1-\sqrt\tau)$.  With $c=c_\vartheta$ the condition
reads $\lambda^h_j<\lambda_\tau$, which gives the count.

(c) Since $s\mapsto s/(s+c_\vartheta)$ is nondecreasing on $(0,\infty)$ and
$\lambda^h_j\ge\lambda^h_1$, all eigenvalues in (a) are at least
$(1+c_\vartheta/\lambda^h_1)^{-2}$, and Lemma~\ref{lem:wm-pencil}(a) turns
this into the first Loewner inequality.  If
$K_0\succeq\underline\lambda M_D$, then $\lambda^h_1\ge\underline\lambda$
by Lemma~\ref{lem:wm-pencil}(a), so
$(1+c_\vartheta/\lambda^h_1)^{-2}\ge(1+c_\vartheta/\underline\lambda)^{-2}
=(1+\varsigma_\vartheta)^{-2}$.
\end{proof}

In the modal basis, the upper end $H_0+\Lambda_L\gamma^{-1}\mathcal M$ of
the enclosure of $P_W$ is compared with $P_\vartheta$ through the following
ratio.

\begin{lemma}[A ratio bound]\label{lem:wm-scalarfn}
Let $\gamma>0$, $\Lambda_L\ge1$, $c\ge0$ and $\ell>0$, and let
$f(s) \coloneqq (s^2+\Lambda_L\gamma^{-1})/(s+c)^2$ for $s>0$.  Then
$f(s)\le\max\{1,f(\ell)\}$ for every $s\ge\ell$.
\end{lemma}

\begin{proof}
A direct computation gives $f'(s)=2(cs-\Lambda_L\gamma^{-1})/(s+c)^3$.  Let
$s\ge\ell$.  If $f(s)\le1$, there is nothing to prove, so let $f(s)>1$.
Then $s^2+\Lambda_L\gamma^{-1}>(s+c)^2$, and hence
$\Lambda_L\gamma^{-1}>2cs+c^2\ge ct$ for every $t\in[\ell,s]$.  Thus
$f'<0$ on $[\ell,s]$, and $f(s)\le f(\ell)$.
\end{proof}

The first theorem compares $P_\vartheta$ with $P_W$ for every mask and,
under a two-sided bound for $H$, with the Newton matrix $J$.

\begin{theorem}[Spectral equivalence]\label{thm:wm-equiv}
Let $\gamma>0$ and $\vartheta\ge0$, assume \eqref{eq:wm-exactquad} and
\eqref{eq:wm-lump}, and define
\[
 \mu_- \coloneqq (1+\varsigma_\vartheta)^{-2},\qquad
 \mu_+ \coloneqq \max\bigl\{1,(1+\Lambda_L\varepsilon_\gamma)
 (1+\varsigma_\vartheta)^{-2}\bigr\}.
\]
\begin{enumerate}[label=\textup{(\alph*)},leftmargin=*]
\item For every diagonal $0\le D\le I_m$, the eigenvalues of
 $P_\vartheta^{-1}P_W$ lie in $[\mu_-,\mu_+]$.  More precisely,
 \begin{equation}\label{eq:wm-scalar-equiv}
  \mu_-P_\vartheta\preceq H_0\preceq P_W\preceq
  H_0+\Lambda_L\gamma^{-1}\mathcal M\preceq\mu_+P_\vartheta .
 \end{equation}
\item Consequently, for every diagonal $0\le D\le I_m$,
 \begin{equation}\label{eq:wm-scalar-kappa}
  \kappa_{\rm sp}(P_\vartheta^{-1}P_W)\le\chi_\gamma(\vartheta),\qquad
  \chi_\gamma(\vartheta)\le\max\{2,\Lambda_L\}(1+\varepsilon_\gamma)
  \quad\text{if }0\le\vartheta\le1.
 \end{equation}
\item Let, in addition, $c_HH_0\preceq H\preceq C_HH_0$ for constants
 $0<c_H\le C_H$, and let $\theta_- \coloneqq \min\{c_H,1\}$ and
 $\theta_+ \coloneqq \max\{C_H,1\}$ be the constants of
 Theorem~\ref{thm:wm-algebra}.  Then, for every diagonal $0\le D\le I_m$,
 \begin{equation}\label{eq:wm-scalar-J}
  \operatorname{spec}(P_\vartheta^{-1}J)\subset[c_H\mu_-,\theta_+\mu_+],
  \qquad
  \kappa_{\rm sp}(P_\vartheta^{-1}J)\le\frac{\theta_+}{c_H}\,
  \chi_\gamma(\vartheta)\le\frac{\theta_+}{\theta_-}\,\chi_\gamma(\vartheta).
 \end{equation}
\item The lower end $\mu_-$ is an eigenvalue of $P_\vartheta^{-1}P_W(D)$
 for some diagonal $0\le D\le I_m$ if and only if $\vartheta=0$ or
 $\underline\lambda=\lambda^h_1$.  It is then an eigenvalue for $D=0$.  If
 $0<\vartheta\le1$, then $\mu_+\le\Lambda_L/\vartheta$, a bound
 independent of $\gamma$.
\item For $D=I_m$ and $\vartheta=1$,
 $\operatorname{spec}(P_1^{-1}P_W)\subset[1/2,\Lambda_L]$, an interval
 independent of $\gamma$.
\end{enumerate}
\end{theorem}

\begin{proof}
We enclose $P_W$ between two matrices that are diagonal in the modal basis
of Lemma~\ref{lem:wm-modal}.  This reduces the comparison with $P_\vartheta$
to scalar inequalities.

(a) By
Lemma~\ref{lem:wm-lump}(c), $0\preceq C_D\preceq\Lambda_L\mathcal M$, hence
$H_0\preceq P_W\preceq H_0+\Lambda_L\gamma^{-1}\mathcal M$.  By
Lemma~\ref{lem:wm-modal}, the congruence with $\widetilde X_h$ maps
$H_0+\Lambda_L\gamma^{-1}\mathcal M$ and $P_\vartheta$ to the diagonal
matrices $I_{n_\xi}\otimes(\Lambda_h^2+\Lambda_L\gamma^{-1}I)$ and
$I_{n_\xi}\otimes(\Lambda_h+c_\vartheta I)^2$.  Since
$\lambda^h_j\ge\underline\lambda$ by \eqref{eq:wm-lump} and
Lemma~\ref{lem:wm-pencil}(a), Lemma~\ref{lem:wm-scalarfn} with
$c=c_\vartheta$ and $\ell=\underline\lambda$ gives, for every $j$,
\[
 \frac{(\lambda^h_j)^2+\Lambda_L\gamma^{-1}}{(\lambda^h_j+c_\vartheta)^2}
 \le\max\Bigl\{1,\frac{\underline\lambda^2+\Lambda_L\gamma^{-1}}
 {(\underline\lambda+c_\vartheta)^2}\Bigr\}
 =\max\Bigl\{1,\frac{1+\Lambda_L\varepsilon_\gamma}
 {(1+\varsigma_\vartheta)^2}\Bigr\}=\mu_+,
\]
where we divided the numerator and the denominator of the middle fraction
by $\underline\lambda^2$.  Hence
$H_0+\Lambda_L\gamma^{-1}\mathcal M\preceq\mu_+P_\vartheta$.  Together
with $\mu_-P_\vartheta\preceq H_0$ from Lemma~\ref{lem:wm-modal}(c), this
proves \eqref{eq:wm-scalar-equiv}, and Lemma~\ref{lem:wm-pencil}(a) turns
it into $\operatorname{spec}(P_\vartheta^{-1}P_W)\subset[\mu_-,\mu_+]$.

(b) By (a),
\[
 \kappa_{\rm sp}(P_\vartheta^{-1}P_W)\le\frac{\mu_+}{\mu_-}
 =\max\bigl\{(1+\varsigma_\vartheta)^2,\,1+\Lambda_L\varepsilon_\gamma\bigr\}
 =\chi_\gamma(\vartheta).
\]
If $0\le\vartheta\le1$, then
\[
 (1+\varsigma_\vartheta)^2\le2(1+\varsigma_\vartheta^2)
 =2(1+\vartheta\varepsilon_\gamma)\le2(1+\varepsilon_\gamma),
\]
and $1+\Lambda_L\varepsilon_\gamma\le\Lambda_L(1+\varepsilon_\gamma)$ since
$\Lambda_L\ge1$.  Hence
$\chi_\gamma(\vartheta)\le\max\{2,\Lambda_L\}(1+\varepsilon_\gamma)$, the
second bound in \eqref{eq:wm-scalar-kappa}.

(c) By Theorem~\ref{thm:wm-algebra} and
Lemma~\ref{lem:wm-pencil}(a), $J\preceq\theta_+P_W$, and hence
$J\preceq\theta_+\mu_+P_\vartheta$ by \eqref{eq:wm-scalar-equiv}.  On the
other side,
$J\succeq H\succeq c_HH_0\succeq c_H\mu_-P_\vartheta$.
Lemma~\ref{lem:wm-pencil}(a) gives the enclosure in \eqref{eq:wm-scalar-J},
and the bounds for $\kappa_{\rm sp}$ follow from
$\theta_+\mu_+/(c_H\mu_-)=(\theta_+/c_H)\chi_\gamma(\vartheta)$ and
$c_H\ge\theta_-$.

(d) Since $C_D\succeq0=C_0$, we have $P_W(D)\succeq P_W(0)=H_0$ for every
$D$.  Hence, by
Lemma~\ref{lem:wm-pencil}(a) and Lemma~\ref{lem:wm-modal}(a),
\[
 \min_D\lambda_{\min}(P_\vartheta^{-1}P_W)
 =\lambda_{\min}(P_\vartheta^{-1}H_0)=(1+c_\vartheta/\lambda^h_1)^{-2},
\]
attained at $D=0$ by every vector $\zeta\otimes g$ with
$0\ne\zeta\in\R^{n_\xi}$ and $0\ne g\in\R^{n_h}$ such that
$K_0g=\lambda^h_1M_Dg$.  By (a), this minimum is at least $\mu_-$.
Hence $\mu_-$ is an eigenvalue for some $D$ if and only if the minimum
equals $\mu_-=(1+c_\vartheta/\underline\lambda)^{-2}$.  This holds if and
only if $c_\vartheta=0$, that is, $\vartheta=0$, or
$\underline\lambda=\lambda^h_1$.
For $0<\vartheta\le1$ we have $(1+\varsigma_\vartheta)^2\ge
1+\varsigma_\vartheta^2=1+\vartheta\varepsilon_\gamma$, so
\[
 \mu_+\le\max\Bigl\{1,\frac{1+\Lambda_L\varepsilon_\gamma}
 {1+\vartheta\varepsilon_\gamma}\Bigr\}
 \le\max\Bigl\{1,\frac{\Lambda_L}{\vartheta}\Bigr\}
 =\frac{\Lambda_L}{\vartheta},
\]
where the second inequality uses $\vartheta\le1\le\Lambda_L$.

(e) We have $C_{I_m}=I_{n_\xi}\otimes M_L$ by
Lemma~\ref{lem:wm-lump}(c).  Hence \eqref{eq:wm-lump},
Lemma~\ref{lem:wm-pencil}(b) and $\Lambda_L\ge1$ give
$H_0+\gamma^{-1}\mathcal M\preceq P_W\preceq
\Lambda_L(H_0+\gamma^{-1}\mathcal M)$.  The matching inequality for
$P_1=P_{\rm mean}$ in Section~\ref{sec:numerics} gives
$H_0+\gamma^{-1}\mathcal M\preceq P_1\preceq
2(H_0+\gamma^{-1}\mathcal M)$.  Together,
$\tfrac12P_1\preceq P_W\preceq\Lambda_LP_1$, and
Lemma~\ref{lem:wm-pencil}(a) gives the claim.
\end{proof}

By Theorem~\ref{thm:wm-equiv}(d), for $0<\vartheta\le1$ the growth of
$\chi_\gamma(\vartheta)=\mu_+/\mu_-$ as $\gamma\to0$ comes from the lower
end $\mu_-=(1+\varsigma_\vartheta)^{-2}$, that is, from small eigenvalues.
For $\vartheta=0$, we have $\mu_-=1$, and the growth comes from the upper
end $\mu_+=1+\Lambda_L\varepsilon_\gamma$.  Under Assumption~\ref{ass:wm-local},
$\lambda_*<2\pi^2\nu_-/d^2<\lambda^h_1$ by Lemma~\ref{lem:wm-weyl}(a), so
for both choices of $\underline\lambda$ the lower end $\mu_-$ is an
eigenvalue only if $\vartheta=0$.  Since parts (a)--(c) of Theorem~\ref{thm:wm-equiv} hold for every
$\vartheta\ge0$ and every mask, they cover the value
$\vartheta=\widehat\vartheta_k$ stored at the last refactorization in
Section~\ref{sec:numerics}.

The proof of Theorem~\ref{thm:wm-count} counts eigenvalues through
inertia, and the next lemma collects the facts it uses.

\begin{lemma}[Inertia counts]\label{lem:wm-inertia}
Let $A=A^\top$ and $B\succ0$ in $\R^{n\times n}$, let $X$, $X'$ and $Y$ be
symmetric $n\times n$ matrices, and let $t\in\R$.
\begin{enumerate}[label=\textup{(\alph*)},leftmargin=*]
\item The counts are $n_{>t}(A,B)=\iota_+(A-tB)$ and
 $n_{<t}(A,B)=\iota_-(A-tB)$.  The number $\iota_+(X)$ (respectively
 $\iota_-(X)$) is the largest dimension of a subspace on which $X$ is
 positive (respectively negative) definite.
\item Let $0\le r\le n$.  If $v^\top Av\le t\,v^\top Bv$ for all $v$ in a
 subspace of dimension at least $n-r$, then $n_{>t}(A,B)\le r$.  If
 $v^\top Av\ge t\,v^\top Bv$ for all $v$ in such a subspace, then
 $n_{<t}(A,B)\le r$.
\item If $X\preceq X'$, then $\iota_+(X)\le\iota_+(X')$ and
 $\iota_-(X)\ge\iota_-(X')$.  Adding $Y$ lowers $\iota_-$ by at most its
 rank: $\iota_-(X+Y)\ge\iota_-(X)-\operatorname{rank}Y$.
\end{enumerate}
\end{lemma}

\begin{proof}
(a) Let $B=LL^\top$ and $C=L^{-1}AL^{-\top}$ be as in the proof of
Lemma~\ref{lem:wm-pencil}(a).  Since $A-tB=L(C-tI)L^\top$, Sylvester's law
of inertia gives
$\iota_\pm(A-tB)=\iota_\pm(C-tI)$, and these are the numbers of eigenvalues
of $C$, and hence of $B^{-1}A$, above and below $t$.  For the second
statement, let $X$ have orthonormal eigenvectors $q_i$ with eigenvalues
$\lambda_i(X)$.  Then $X$ is positive definite on
$\operatorname{span}\{q_i:\lambda_i(X)>0\}$, whose dimension is
$\iota_+(X)$.  Every subspace of larger dimension meets
$\operatorname{span}\{q_i:\lambda_i(X)\le0\}$ in a nonzero vector $v$, for
which $v^\top Xv\le0$.  Applying this to $-X$ gives the statement for
$\iota_-(X)$.

(b) Let $\mathcal S_0$ be the given subspace.  The matrix $A-tB$ is
negative semidefinite on $\mathcal S_0$, so every subspace on which $A-tB$
is positive definite meets $\mathcal S_0$ only in $0$ and therefore has
dimension at most $n-\dim\mathcal S_0\le r$.  By (a),
$n_{>t}(A,B)=\iota_+(A-tB)\le r$.  The second statement follows by applying
the first one to $(-A,B)$ and the threshold $-t$, because
$n_{>-t}(-A,B)=n_{<t}(A,B)$.

(c) If $X\preceq X'$, then a subspace on which $X$ is positive definite is
one on which $X'$ is positive definite, and a subspace on which $X'$ is
negative definite is one on which $X$ is negative definite.  The
second statement of (a) gives the claim.  For the last statement, let $X$ be negative
definite on a subspace $\mathcal S$ with $\dim\mathcal S=\iota_-(X)$.  Then
$X+Y$ is negative definite on $\mathcal S\cap\ker Y$, whose dimension is
at least $\iota_-(X)-\operatorname{rank}Y$, and (a) gives the claim.
\end{proof}

On the meshes of Assumption~\ref{ass:wm-local}, the number of small
eigenvalues $\lambda^h_j$ is bounded through the explicit spectrum of the
uniform $Q_1$ discretization.  We recall
from the proof of
Lemma~\ref{lem:wm-reference} the one-dimensional interior mass and
stiffness matrices, their eigenvalues for the sine vectors
$(\sin(ir\pi/n_e))_{i=1}^{n_e-1}$, $1\le r\le n_e-1$, and the tensor
identities:
\begin{gather*}
 M_1=\frac h6\operatorname{tridiag}(1,4,1),\qquad
 S_1=\frac1h\operatorname{tridiag}(-1,2,-1),\\
 m_r=\frac h3(2+\cos\theta_r),\qquad s_r=\frac2h(1-\cos\theta_r),\qquad
 \theta_r=\frac{r\pi}{n_e},\\
 M_D=M_1\otimes M_1,\qquad K_{\rm unit}=M_1\otimes S_1+S_1\otimes M_1,\qquad
 K_0\succeq\nu_-K_{\rm unit},
\end{gather*}
where $K_{\rm unit}$ is the stiffness matrix for $a_{0,Tq}\equiv1$.  Its
tensor form holds because the $2\times2$ Gauss rule integrates the bilinear
stiffness exactly on the square elements.  The
function $\Theta$ of the next lemma satisfies
$s_r/m_r=h^{-2}\Theta(\theta_r)$.  The number $h^{-2}\Theta(\theta_r)$ is
the $r$th eigenvalue of the one-dimensional discrete Dirichlet Laplacian
$M_1^{-1}S_1$ on an interval of length $d$.  The number
$h^{-2}\theta_r^2=(r\pi/d)^2$ is the $r$th eigenvalue of $-v''=\lambda v$
on that interval with $v=0$ at both ends.  The inequality
$\Theta(\theta)\ge\theta^2$ thus states that the discrete eigenvalues lie
above the continuous ones, as the min--max principle predicts for a
conforming Galerkin discretization.  Lemma~\ref{lem:wm-theta} proves it
directly, with strict inequality for $\theta>0$.  This gives the strict
bound in Lemma~\ref{lem:wm-weyl}(a).

\begin{lemma}[A trigonometric inequality]\label{lem:wm-theta}
The function
\[
 \Theta(\theta) \coloneqq \frac{6(1-\cos\theta)}{2+\cos\theta}
\]
satisfies $\Theta(\theta)\ge\theta^2$ for $0\le\theta\le\pi$, with equality
only at $\theta=0$.
\end{lemma}

\begin{proof}
Define $u \coloneqq \theta/2\in[0,\pi/2]$.  Then
$1-\cos\theta=2\sin^2u$ and $2+\cos\theta=\sin^2u+3\cos^2u$, so the claim
$\Theta(\theta)\ge4u^2$ is equivalent to
\[
 (3-u^2)\sin^2u\ge3u^2\cos^2u .
\]
At $u=0$ both sides vanish, and at $u=\pi/2$ the inequality reads
$3-\pi^2/4>0$.  Let $0<u<\pi/2$ and $t \coloneqq u^2/3\in(0,\pi^2/12)\subset(0,5/6)$.
After division by $3\cos^2u$ the claim becomes $(1-t)\tan^2u\ge u^2$.  We
show that this holds strictly.

The functions $\tan u-u$,
$\tan u-u-u^3/3$ and $\tan u-u-u^3/3-2u^5/15$ vanish at $u=0$, and their
derivatives are
\[
 \tan^2u,\qquad\tan^2u-u^2,\qquad
 \tan^2u-u^2-\tfrac23u^4\ge\bigl(u+\tfrac13u^3\bigr)^2-u^2-\tfrac23u^4
 =\tfrac19u^6 .
\]
The first derivative is nonnegative.  Each of the other two is
nonnegative because the preceding function is nonnegative, that is,
because $\tan u\ge u\ge0$, respectively $\tan u\ge u+u^3/3\ge0$.  Hence
\[
 \tan u\ge u+\frac{u^3}{3}+\frac{2u^5}{15}
 =u\Bigl(1+t+\frac65t^2\Bigr)>0 .
\]

%\emph{Step 3 (a polynomial inequality).}  
Since $1-t>0$, this gives
\[
 (1-t)\tan^2u\ge u^2\Bigl(1+t+\frac65t^2\Bigr)^2(1-t)
 =u^2\bigl(1+t\,p(t)\bigr),
\]
where
\[
 p(t) \coloneqq 1+\frac75t-t^2-\frac{24}{25}t^3-\frac{36}{25}t^4 .
\]
Since $p''(t)=-2-(144/25)t-(432/25)t^2<0$ for $t\ge0$, the
polynomial $p$ is concave on $[0,5/6]$, so
$p\ge\min\{p(0),p(5/6)\}=\min\{1,2/9\}>0$ there.  Thus
$(1-t)\tan^2u>u^2$ for $0<u<\pi/2$.
\end{proof}

The next lemma bounds $\lambda^h_1$ from below and $\mathcal N_h$ from
above.  It gives the value $\underline\lambda=2\pi^2\nu_-/d^2$ and the
$h$-independent count in Theorem~\ref{thm:wm-count}(iv).

\begin{lemma}[Spectrum of the mean stiffness]\label{lem:wm-weyl}
Let Assumption~\ref{ass:wm-local} hold.
\begin{enumerate}[label=\textup{(\alph*)},leftmargin=*]
\item The smallest eigenvalue satisfies $\lambda^h_1>2\pi^2\nu_-/d^2$.  Thus
 $\underline\lambda=2\pi^2\nu_-/d^2$ is admissible in \eqref{eq:wm-lump}.
\item The counting function satisfies
 $\mathcal N_h(\lambda)\le d^2\lambda/(4\pi\nu_-)$ for every
 $\lambda\ge0$, and it vanishes for $\lambda\le2\pi^2\nu_-/d^2$.
\end{enumerate}
\end{lemma}

The bound in (b) is the leading term of Weyl's law for the number of
Dirichlet eigenvalues of $-\nu_-\Delta$ below $\lambda$ on a square of side
$d$.  Here it bounds the discrete count for every $\lambda$ and every $h$.

\begin{proof}
% \emph{Step 1 (explicit spectrum).}  
The tensor products of the sine vectors
diagonalize $M_D=M_1\otimes M_1$ and
$K_{\rm unit}=M_1\otimes S_1+S_1\otimes M_1$.  Hence the eigenvalues of
$M_D^{-1}K_{\rm unit}$, with multiplicity, are
\[
 \frac{s_i}{m_i}+\frac{s_l}{m_l}
 =h^{-2}\bigl(\Theta(\theta_i)+\Theta(\theta_l)\bigr),\qquad
 1\le i,l\le n_e-1 .
\]
Since $\theta_i/h=i\pi/d$ and $0<\theta_i<\pi$, Lemma~\ref{lem:wm-theta}
gives
\[
 h^{-2}\bigl(\Theta(\theta_i)+\Theta(\theta_l)\bigr)
 >\frac{\pi^2(i^2+l^2)}{d^2}.
\]

Then every eigenvalue of
$M_D^{-1}K_{\rm unit}$ exceeds $\min_{i,l\ge1}\pi^2(i^2+l^2)/d^2=2\pi^2/d^2$.
Since $K_0\succeq\nu_-K_{\rm unit}$, Lemma~\ref{lem:wm-pencil}(a) gives
$\lambda^h_1\ge\nu_-\lambda_1(K_{\rm unit},M_D)>2\pi^2\nu_-/d^2$, which
proves (a).

Let $\lambda\ge0$.  Since
$K_0-\lambda M_D\succeq\nu_-K_{\rm unit}-\lambda M_D$, parts (a) and (c)
of Lemma~\ref{lem:wm-inertia} and the explicit eigenvalues of
$M_D^{-1}K_{\rm unit}$ above give
\begin{align*}
 \mathcal N_h(\lambda)&=\iota_-(K_0-\lambda M_D)
 \le\iota_-(\nu_-K_{\rm unit}-\lambda M_D)\\
 &=\#\bigl\{(i,l):\nu_-h^{-2}\bigl(\Theta(\theta_i)+\Theta(\theta_l)\bigr)
  <\lambda\bigr\}\\
 &\le\#\bigl\{(i,l):\pi^2(i^2+l^2)/d^2<\lambda/\nu_-\bigr\}\le L(R),
\end{align*}
where $R^2 \coloneqq \lambda d^2/(\pi^2\nu_-)$ and
$L(R) \coloneqq \#\{(i,l)\in\mathbb Z^2:i,l\ge1,\ i^2+l^2<R^2\}$.  The half-open
unit squares $(i-1,i]\times(l-1,l]$ of the counted pairs are pairwise
disjoint and lie in the open quarter disk
$\{z\in\R^2:z_1,z_2>0,\ |z|<R\}$, so $L(R)\le\pi R^2/4=d^2\lambda/(4\pi\nu_-)$.
By (a), $\mathcal N_h(\lambda)=0$ for $\lambda\le2\pi^2\nu_-/d^2$.  This
proves (b).
\end{proof}

The second theorem counts the eigenvalues of $P_\vartheta^{-1}P_W$ outside
$[\tau,1]$.

\begin{theorem}[Outlying eigenvalues]\label{thm:wm-count}
Let $\gamma>0$, $\vartheta\ge0$ and $0<\tau<1$, and let
$\lambda_\tau=c_\vartheta\sqrt\tau/(1-\sqrt\tau)$ be as in
Lemma~\ref{lem:wm-modal}(b).  In \textup{(i)} and \textup{(ii)}, $C_D$ is
any symmetric positive semidefinite $N\times N$ matrix,
$P_W=H_0+\gamma^{-1}C_D$ and $J=H+\gamma^{-1}C_D$.  The statements
about $J$ assume $c_HH_0\preceq H\preceq C_HH_0$ for constants
$0<c_H\le C_H$.  By \textup{(i)} and \textup{(ii)}, all but at most
$\operatorname{rank}C_D+n_\xi\mathcal N_h(\lambda_\tau)$ eigenvalues of
$P_\vartheta^{-1}P_W$ lie in $[\tau,1]$.  Parts \textup{(iii)} and
\textup{(iv)} bound $\operatorname{rank}C_D$ and
$\mathcal N_h(\lambda_\tau)$.
\begin{enumerate}[label=\textup{(\roman*)},leftmargin=*]
\item At most $\operatorname{rank}C_D$ eigenvalues of
 $P_\vartheta^{-1}P_W$ exceed $1$, and exactly $\operatorname{rank}C_D$ of
 them do if $\vartheta=0$.  At most $\operatorname{rank}C_D$ eigenvalues
 of $P_\vartheta^{-1}J$ exceed $C_H$.
\item The number $n_\tau$ of eigenvalues of $P_\vartheta^{-1}P_W$ below
 $\tau$ satisfies
 \begin{equation}\label{eq:wm-scalar-count}
  n_\xi\mathcal N_h(\lambda_\tau)-\operatorname{rank}C_D\le n_\tau
  \le n_\xi\mathcal N_h(\lambda_\tau),
 \end{equation}
 with equality on the right if $C_D=0$.  At most
 $n_\xi\mathcal N_h(\lambda_\tau)$ eigenvalues of $P_\vartheta^{-1}J$ lie
 below $c_H\tau$, and at least
 $n_\xi\mathcal N_h(\lambda_\tau)-\operatorname{rank}C_D$ lie below
 $C_H\tau$.
\item For $C_D=E^\top WDE$ with a diagonal $0\le D\le I_m$, let
 $\mathcal F_r \coloneqq \{k:D_{(k,r)}>0\}$ collect
 the quadrature points at which the control value at $x_r$ is free, and
 let $V_\xi[\mathcal F_r]$ consist of the rows $k\in\mathcal F_r$ of
 $V_\xi$.  Then
 \[
  \operatorname{rank}C_D=\sum_{r=1}^{n_h}\operatorname{rank}
  V_\xi[\mathcal F_r]\le\min\Bigl\{\sum_{r=1}^{n_h}|\mathcal F_r|,\;
  n_\xi\,\#\{r:\mathcal F_r\ne\emptyset\}\Bigr\}.
 \]
 For a binary mask, $\sum_r|\mathcal F_r|=\operatorname{Tr}D$ is the
 number of free control values.
\item Under Assumption~\ref{ass:wm-local},
 $\mathcal N_h(\lambda)\le d^2\lambda/(4\pi\nu_-)$ for every $\lambda\ge0$
 and every $h$, and $\mathcal N_h(\lambda)=0$ for
 $\lambda\le2\pi^2\nu_-/d^2$.
\end{enumerate}
\end{theorem}

\begin{proof}
Parts (i) and (ii) compare $P_\vartheta^{-1}P_W$ with $P_\vartheta^{-1}H_0$,
whose counts are known.  Since
$P_\vartheta-H_0=2c_\vartheta\overline{\mathcal K}+c_\vartheta^2\mathcal M
\succeq0$ by \eqref{eq:wm-Ptheta}, no eigenvalue of $P_\vartheta^{-1}H_0$
exceeds $1$, and Lemma~\ref{lem:wm-modal}(b) counts those below $\tau$.  Adding
$\gamma^{-1}C_D$ changes each count by at most $\operatorname{rank}C_D$.

(i) On $\ker C_D$, a subspace of dimension $N-\operatorname{rank}C_D$, we
have $v^\top P_Wv=v^\top H_0v\le v^\top P_\vartheta v$ and
$v^\top Jv=v^\top Hv\le C_Hv^\top H_0v\le C_Hv^\top P_\vartheta v$.
Lemma~\ref{lem:wm-inertia}(b), with $r=\operatorname{rank}C_D$ and $t=1$,
respectively $t=C_H$, gives both upper bounds.  If $\vartheta=0$, then
$P_W-P_0=\gamma^{-1}C_D$ has exactly $\operatorname{rank}C_D$ positive
eigenvalues, so Lemma~\ref{lem:wm-inertia}(a) gives
$n_{>1}(P_W,P_0)=\operatorname{rank}C_D$.

(ii) By Lemma~\ref{lem:wm-inertia}(a) and Lemma~\ref{lem:wm-modal}(b),
$\iota_-(H_0-\tau P_\vartheta)=n_\xi\mathcal N_h(\lambda_\tau)$.  Since
\[
 P_W-\tau P_\vartheta=(H_0-\tau P_\vartheta)+\gamma^{-1}C_D
 \succeq H_0-\tau P_\vartheta,
\]
Lemma~\ref{lem:wm-inertia}(a),(c) gives
\[
 n_\xi\mathcal N_h(\lambda_\tau)-\operatorname{rank}C_D\le n_\tau
 =\iota_-(P_W-\tau P_\vartheta)\le n_\xi\mathcal N_h(\lambda_\tau),
\]
with equality on the right for $C_D=0$.  For $J$, the relation
$J-c_H\tau P_\vartheta\succeq c_H(H_0-\tau P_\vartheta)$ gives
$n_{<c_H\tau}(J,P_\vartheta)\le\iota_-(H_0-\tau P_\vartheta)$.  The
relation $J-C_H\tau P_\vartheta\preceq C_H(H_0-\tau P_\vartheta)
+\gamma^{-1}C_D$ gives
\[
 n_{<C_H\tau}(J,P_\vartheta)
 \ge\iota_-\bigl(C_H(H_0-\tau P_\vartheta)+\gamma^{-1}C_D\bigr)
 \ge\iota_-(H_0-\tau P_\vartheta)-\operatorname{rank}C_D .
\]

(iii) Since $W$ and $D$ are diagonal with $W\succ0$ and $D\ge0$, we have
$C_D=(W^{1/2}D^{1/2}E)^\top(W^{1/2}D^{1/2}E)$, so
$\operatorname{rank}C_D=\operatorname{rank}(W^{1/2}D^{1/2}E)
=\operatorname{rank}(D^{1/2}E)$.  The row of $D^{1/2}E$ with index $(k,r)$
is $D_{(k,r)}^{1/2}\,(\psi(\xi_k)^\top\otimes e_r^\top)$, where
$\psi(\xi_k) \coloneqq (\psi_j(\xi_k))_{j=1}^{n_\xi}$ and $e_r$ is the $r$th unit
vector of $\R^{n_h}$.  This row vanishes for $k\notin\mathcal F_r$.  Hence the row
space of $D^{1/2}E$ is
\[
 \bigoplus_{r=1}^{n_h}\operatorname{span}\{\psi(\xi_k):k\in\mathcal F_r\}
 \otimes e_r,
\]
a direct sum of subspaces of the mutually orthogonal spaces
$\R^{n_\xi}\otimes e_r$.  Its dimension is
$\sum_r\operatorname{rank}V_\xi[\mathcal F_r]$.  The bounds follow from
$\operatorname{rank}V_\xi[\mathcal F_r]\le\min\{|\mathcal F_r|,n_\xi\}$,
and for a binary mask $\sum_r|\mathcal F_r|=\operatorname{Tr}D$.

(iv) This is Lemma~\ref{lem:wm-weyl}(b).
\end{proof}

The third theorem works on a model problem.  Let
Assumption~\ref{ass:wm-local} hold on the square $(-d/2,d/2)^2$ with
$n_e\ge3$ elements per direction and a constant mean coefficient,
$a_{0,Tq}\equiv\nu>0$.  Let
$\mathcal O_\pm \coloneqq \{x\in(-d/2,d/2)^2:\pm x_1>0\}$ be the right and
the left half of the square, let $\Pi_\pm\in\R^{n_h\times n_h}$ be the
diagonal matrix with $(\Pi_\pm)_{rr}=1$ if $x_r\in\mathcal O_\pm$ and
$(\Pi_\pm)_{rr}=0$ otherwise, and let $D^\pm \coloneqq I_{n_q}\otimes\Pi_\pm$.
These two binary masks are mirror images of each other.  The mask
$D^\pm$ is free exactly at the points $(x_r,\xi_k)$ with $x_r\in\mathcal O_\pm$.  Define
\begin{equation}\label{eq:wm-varrho}
 \varrho_h \coloneqq \min\Bigl\{\frac{g^\top K_0M_D^{-1}K_0\,g}{g^\top M_D\,g}:
 0\ne g\in\R^{n_h},\ \Pi_+g=g\Bigr\}.
\end{equation}

The next lemma is the triangle inequality for Hilbert's projective metric
on SPD matrices, whose value at $(A,B)$ is the logarithm of
$\kappa_{\rm sp}(A^{-1}B)$.  In the proof of Theorem~\ref{thm:wm-obstr}
it turns a lower bound for the distance between
$P_W(D^+)$ and $P_W(D^-)$ into a lower bound for the larger of the
distances from an arbitrary SPD matrix $Q$ to these two matrices.

\begin{lemma}[Hilbert-metric inequality]\label{lem:wm-hilbert}
For SPD matrices $A$, $B$ and $Q$ of equal size,
\[
 \kappa_{\rm sp}(A^{-1}B)\le\kappa_{\rm sp}(Q^{-1}A)\,
 \kappa_{\rm sp}(Q^{-1}B).
\]
\end{lemma}

\begin{proof}
Let $a_-\le a_+$ and $b_-\le b_+$ be the extreme eigenvalues of $Q^{-1}A$
and $Q^{-1}B$, respectively.  By Lemma~\ref{lem:wm-pencil}(a),
$a_-Q\preceq A\preceq a_+Q$ and $b_-Q\preceq B\preceq b_+Q$.  Hence
\[
 \frac{b_-}{a_+}\,A\preceq b_-Q\preceq B\preceq b_+Q
 \preceq\frac{b_+}{a_-}\,A .
\]
By Lemma~\ref{lem:wm-pencil}(a) again,
$\operatorname{spec}(A^{-1}B)\subset[b_-/a_+,b_+/a_-]$, and therefore
$\kappa_{\rm sp}(A^{-1}B)\le(b_+/b_-)(a_+/a_-)
=\kappa_{\rm sp}(Q^{-1}B)\,\kappa_{\rm sp}(Q^{-1}A)$.
\end{proof}

The next lemma shows that the reflection $x_1\mapsto-x_1$ exchanges the
masks $D^+$ and $D^-$ while leaving $H_0$ and every $P_\vartheta$
unchanged.  It also shows that on suitable subspaces each of $P_W(D^+)$
and $P_W(D^-)$ dominates the other by the factor $1+(\gamma\varrho_h)^{-1}$.

\begin{lemma}[Mirror masks]\label{lem:wm-mirror}
Let $a_{0,Tq}\equiv\nu>0$ and let Assumption~\ref{ass:wm-local} hold on the
square $(-d/2,d/2)^2$ with $n_e\ge3$, assume \eqref{eq:wm-exactquad}, let
$\gamma>0$, and let $\Pi_\pm$ and $D^\pm$ be as defined before
\eqref{eq:wm-varrho} and $\varrho_h$ as in \eqref{eq:wm-varrho}.  Order the
interior nodes $x_r=(t_i,t_l)$, $t_i=-d/2+ih$, $1\le i,l\le n_e-1$,
lexicographically with $i$ running fastest.  Let
$\mathsf R\in\R^{(n_e-1)\times(n_e-1)}$ be the exchange matrix, which
reverses the order of the entries of a vector, and put
$\mathsf F \coloneqq I_{n_e-1}\otimes\mathsf R$ and
$\widetilde{\mathsf F} \coloneqq I_{n_\xi}\otimes\mathsf F$.  These are symmetric
permutation matrices, equal to their own inverses.
\begin{enumerate}[label=\textup{(\alph*)},leftmargin=*]
\item The active-set terms of the two masks are
 $C_{D^\pm}=I_{n_\xi}\otimes(M_L\Pi_\pm)$.
\item The permutation $\mathsf F$ realizes the reflection of the nodes:
 $(\mathsf Fg)_r=g_{r'}$, where the node $x_{r'}$ is the mirror image
 $(-x_{r,1},x_{r,2})$ of $x_r$.  The reflection leaves the spatial
 matrices invariant and exchanges the two masks:
 \[
  \mathsf FM_D\mathsf F^\top=M_D,\qquad
  \mathsf FK_0\mathsf F^\top=K_0,\qquad
  \mathsf FM_L\mathsf F^\top=M_L,\qquad
  \mathsf F\Pi_+\mathsf F^\top=\Pi_- .
 \]
 Hence, for every $\vartheta\ge0$,
 \[
  \widetilde{\mathsf F}H_0\widetilde{\mathsf F}^\top=H_0,\qquad
  \widetilde{\mathsf F}P_\vartheta\widetilde{\mathsf F}^\top=P_\vartheta,
  \qquad
  \widetilde{\mathsf F}P_W(D^+)\widetilde{\mathsf F}^\top=P_W(D^-).
 \]
\item Let $g_+$ attain the minimum in \eqref{eq:wm-varrho}, put
 $g_- \coloneqq \mathsf Fg_+$ and $\omega_\gamma \coloneqq 1+(\gamma\varrho_h)^{-1}$, and let
 $\mathcal V_\pm \coloneqq \{\zeta\otimes g_\pm:\zeta\in\R^{n_\xi}\}$.  Then
 \begin{alignat*}{2}
  v^\top P_W(D^+)v&\ge\omega_\gamma\,v^\top P_W(D^-)v&\qquad
  &\text{for }v\in\mathcal V_+,\\
  v^\top P_W(D^-)v&\ge\omega_\gamma\,v^\top P_W(D^+)v&
  &\text{for }v\in\mathcal V_-.
 \end{alignat*}
 If $H\preceq C_HH_0$ and $\omega_\gamma^J \coloneqq 1+(\gamma C_H\varrho_h)^{-1}$,
 the same inequalities hold with $J(D^\pm)$ in place of $P_W(D^\pm)$ and
 $\omega_\gamma^J$ in place of $\omega_\gamma$.
\end{enumerate}
\end{lemma}

\begin{proof}
We first show that the minimum in \eqref{eq:wm-varrho} exists and is
positive.  The set $\mathcal O_+$ contains interior nodes because
$n_e\ge3$.  Restricted to the coordinates $r$ with $x_r\in\mathcal O_+$,
the quotient in \eqref{eq:wm-varrho} equals $v^\top A_+v/v^\top B_+v$,
where $A_+$ and $B_+$ are the principal submatrices of $K_0M_D^{-1}K_0$ and
$M_D$ for these coordinates.  Both are SPD.  By
Lemma~\ref{lem:wm-pencil}(a), the minimum is attained and equals
$\lambda_1(A_+,B_+)>0$.

(a) We have $WD^\pm=(W_\xi\otimes M_L)(I_{n_q}\otimes\Pi_\pm)
=W_\xi\otimes(M_L\Pi_\pm)$, and hence, by \eqref{eq:wm-exactquad},
\begin{align*}
 C_{D^\pm}&=(V_\xi^\top\otimes I_{n_h})\bigl(W_\xi\otimes(M_L\Pi_\pm)\bigr)
 (V_\xi\otimes I_{n_h})\\
 &=(V_\xi^\top W_\xi V_\xi)\otimes(M_L\Pi_\pm)
 =I_{n_\xi}\otimes(M_L\Pi_\pm).
\end{align*}

(b) Since $t_{n_e-i}=-t_i$, the permutation $\mathsf F$ maps $(t_i,t_l)$
to $(-t_i,t_l)$, and therefore $\mathcal O_+$ onto $\mathcal O_-$.  By the
proof of Lemma~\ref{lem:wm-reference} and $a_{0,Tq}\equiv\nu$,
$M_D=M_1\otimes M_1$ and $K_0=\nu K_{\rm unit}=\nu(M_1\otimes S_1+S_1\otimes
M_1)$.  Symmetric tridiagonal Toeplitz matrices are persymmetric, that is,
$\mathsf RM_1\mathsf R=M_1$ and $\mathsf RS_1\mathsf R=S_1$, which gives the
first two identities.  For a permutation matrix,
$\mathsf F\operatorname{diag}(u)\mathsf F^\top=\operatorname{diag}(\mathsf Fu)$.
Hence, by $\mathsf F^\top\mathsf F=I$ and $\mathsf F\bm 1=\bm 1$,
\[
 \mathsf FM_L\mathsf F^\top
 =\operatorname{diag}(\mathsf FM_D\mathsf F^\top\mathsf F\bm 1)
 =\operatorname{diag}(M_D\bm 1)=M_L,
\]
and $\mathsf F\Pi_+\mathsf F^\top=\Pi_-$ because $\mathsf F$ maps
$\mathcal O_+$ onto $\mathcal O_-$.  The statements about
$\widetilde{\mathsf F}$ follow from the Kronecker forms
$H_0=I_{n_\xi}\otimes K_0M_D^{-1}K_0$ and \eqref{eq:wm-Ptheta}, and from
$P_W(D^\pm)=H_0+\gamma^{-1}I_{n_\xi}\otimes(M_L\Pi_\pm)$, which is (a).

(c) Let $v=\zeta\otimes g_+$ with $\zeta\in\R^{n_\xi}$.  Since
$\Pi_-g_+=0$, part (a) gives $C_{D^-}v=0$, and
hence
\[
 v^\top P_W(D^-)v=v^\top H_0v=\|\zeta\|_2^2\,g_+^\top K_0M_D^{-1}K_0g_+
 =\|\zeta\|_2^2\,\varrho_h\,g_+^\top M_Dg_+ .
\]
Since $\Pi_+g_+=g_+$ and $M_L\succeq M_D$ by Lemma~\ref{lem:wm-lump}(a),(b),
we have
\[
 v^\top C_{D^+}v=\|\zeta\|_2^2\,g_+^\top M_Lg_+
 \ge\|\zeta\|_2^2\,g_+^\top M_Dg_+,
\]
and therefore
\[
 v^\top P_W(D^+)v\ge\|\zeta\|_2^2\,(\varrho_h+\gamma^{-1})\,g_+^\top M_Dg_+
 =\omega_\gamma\,v^\top P_W(D^-)v .
\]
The inequality on $\mathcal V_-$ follows by applying
$\widetilde{\mathsf F}$: it maps $\mathcal V_+$ onto $\mathcal V_-$, since
$\widetilde{\mathsf F}(\zeta\otimes g_+)=\zeta\otimes g_-$, and by (b) it
exchanges $P_W(D^+)$ and $P_W(D^-)$.

For $J$, let again $v=\zeta\otimes g_+$.  Then
$v^\top J(D^-)v=v^\top Hv$ and
\[
 v^\top Hv\le C_Hv^\top H_0v=C_H\|\zeta\|_2^2\,\varrho_h\,g_+^\top M_Dg_+,
\]
so that
\[
 v^\top J(D^+)v=v^\top Hv+\gamma^{-1}v^\top C_{D^+}v
 \ge v^\top Hv+\frac{v^\top Hv}{\gamma C_H\varrho_h}
 =\omega_\gamma^J\,v^\top J(D^-)v .
\]
Since $H$ need not be invariant under $\widetilde{\mathsf F}$, the
inequality on $\mathcal V_-$ is not obtained by reflection.  The same
computation applies to $v=\zeta\otimes g_-$, using $\Pi_+g_-=0$,
$\Pi_-g_-=g_-$, $g_-^\top M_Dg_-=g_+^\top M_Dg_+$ and
$\widetilde{\mathsf F}H_0\widetilde{\mathsf F}^\top=H_0$.
\end{proof}

The last two lemmas bound $\varrho_h$ from above by means of an explicit
test vector, and the first of them collects the one-dimensional identities
used for it.

\begin{lemma}%[One-dimensional identities]
\label{lem:wm-oned}
Let $n_e\ge2$, $h=d/n_e$ and $t_i=-d/2+ih$.  Let $\hat\phi_i$,
$1\le i\le n_e-1$, be the hat functions of the interior nodes $t_i$ of
$(-d/2,d/2)$, let $V^1_h$ be their span, let $(\cdot,\cdot)$ and
$\|\cdot\|$ be the inner product and the norm of $L^2(-d/2,d/2)$, and let
$P^1_h$ be the $L^2$-orthogonal projection onto $V^1_h$.  Integrals
without limits are over $(-d/2,d/2)$.  The matrices $M_1$ and $S_1$ are the
Gram matrices $(\int\hat\phi_i\hat\phi_k\,dt)_{i,k}$ and
$(\int\hat\phi_i'\hat\phi_k'\,dt)_{i,k}$.  Let
$\Phi\in H^2(-d/2,d/2)$ with $\Phi(\pm d/2)=0$, $\hat a \coloneqq (\Phi(t_i))_i$ and
$I^1_h\Phi \coloneqq \sum_i\hat a_i\hat\phi_i$.
\begin{enumerate}[label=\textup{(\alph*)},leftmargin=*]
\item The interpolant satisfies $\hat a^\top M_1\hat a=\|I^1_h\Phi\|^2$ and
 $\hat a^\top S_1\hat a=\|(I^1_h\Phi)'\|^2\le\|\Phi'\|^2$.
\item The double-stiffness form satisfies
 $\hat a^\top S_1M_1^{-1}S_1\hat a=\|P^1_h\Phi''\|^2\le\|\Phi''\|^2$.
\item The interpolation error satisfies
 $\|\Phi-I^1_h\Phi\|\le(h/\pi)^2\|\Phi''\|$.
\item The vector $\hat b$ with entries
 $\hat b_l=\cos(\pi t_l/d)=\sin(l\pi/n_e)$ satisfies
 $S_1\hat b=\varpi_hM_1\hat b$ with $\varpi_h \coloneqq h^{-2}\Theta(\pi/n_e)$, and
 $\varpi_h\le\eta_h(\pi/d)^2$, where
 $\eta_h \coloneqq (1-\pi^2h^2/(6d^2))^{-1}$.
\end{enumerate}
\end{lemma}

\begin{proof}
The identification of $M_1$ and $S_1$ with these Gram matrices is the
standard computation of the one-dimensional mass and stiffness matrices.
Let $e \coloneqq \Phi-I^1_h\Phi$.  It vanishes at all nodes, including $\pm d/2$.
For an element $T_k \coloneqq [t_{k-1},t_k]$, let $\|\cdot\|_{T_k}$ be the norm of
$L^2(T_k)$.

(a) On every element $T_k$ the functions $(I^1_h\Phi)'$ and $\hat\phi_i'$
are constant, and $\int_{T_k}e'\,dt=e(t_k)-e(t_{k-1})=0$.  Hence
$\int(I^1_h\Phi)'e'\,dt=0$ and $\int e'\hat\phi_i'\,dt=0$ for every $i$.
The first relation gives $\|\Phi'\|^2=\|(I^1_h\Phi)'\|^2+\|e'\|^2$, and (a)
follows, because $\hat a^\top M_1\hat a$ and $\hat a^\top S_1\hat a$ are the
squared norms of $I^1_h\Phi$ and of its derivative.

(b) By the second relation in the proof of (a) and an integration by
parts on $[t_{i-1},t_{i+1}]$, where $\hat\phi_i$ vanishes at both ends and
$\Phi'$ is absolutely continuous,
\[
 (S_1\hat a)_i=\int(I^1_h\Phi)'\hat\phi_i'\,dt=\int\Phi'\hat\phi_i'\,dt
 =-\int\Phi''\hat\phi_i\,dt\eqqcolon-c_i .
\]
With $c \coloneqq (c_i)_i$, the Cauchy--Schwarz inequality in the $M_1$-inner
product and the substitution $v=\sum_i\beta_i\hat\phi_i$ give
\begin{align*}
 \hat a^\top S_1M_1^{-1}S_1\hat a=c^\top M_1^{-1}c
 &=\max_{\beta\ne0}\frac{(c^\top\beta)^2}{\beta^\top M_1\beta}\\
 &=\max_{0\ne v\in V^1_h}\frac{(\Phi'',v)^2}{\|v\|^2}
 =\|P^1_h\Phi''\|^2\le\|\Phi''\|^2 .
\end{align*}

(c) On each $T_k$ we have $e\in H^2(T_k)$, $e=0$ at both endpoints and
$e''=\Phi''$.  Hence $\|e'\|_{T_k}^2=-\int_{T_k}ee''\,dt\le\|e\|_{T_k}
\|\Phi''\|_{T_k}$, and the Friedrichs inequality
$\|e\|_{T_k}\le(h/\pi)\|e'\|_{T_k}$ yields
$\|e\|_{T_k}\le(h/\pi)^2\|\Phi''\|_{T_k}$.  Summing the squares over $k$
gives (c).

(d) Since $t_l=-d/2+lh$, we have $\cos(\pi t_l/d)=\cos(-\pi/2+l\pi/n_e)
=\sin(l\pi/n_e)$.  Thus $\hat b$ is the first sine vector in the proof of
Lemma~\ref{lem:wm-reference}, so $M_1\hat b=m_1\hat b$ and
$S_1\hat b=s_1\hat b$ with
$s_1/m_1=h^{-2}\Theta(\pi/n_e)$.  With $\theta \coloneqq \pi/n_e=\pi h/d$, the
bounds $1-\cos\theta\le\theta^2/2$ and $2+\cos\theta\ge3-\theta^2/2>0$
give
\[
 \varpi_h=\frac{6(1-\cos\theta)}{h^2(2+\cos\theta)}
 \le\frac{3\theta^2}{h^2(3-\theta^2/2)}
 =\frac{\theta^2/h^2}{1-\theta^2/6}=\eta_h\Bigl(\frac\pi d\Bigr)^2 .
\]
\end{proof}

The next lemma gives the upper bound for $\varrho_h$, which for $n_e\ge8$
is an $h$-independent constant $\bar\varrho$.

\begin{lemma}[Upper bound for $\varrho_h$]\label{lem:wm-rho}
Let Assumption~\ref{ass:wm-local} hold on the square $(-d/2,d/2)^2$ with
$n_e\ge4$ and $a_{0,Tq}\equiv\nu>0$, let $\varrho_h$ be as in
\eqref{eq:wm-varrho}, let
$\eta_h$ be as in Lemma~\ref{lem:wm-oned}(d), and put
$\delta_h \coloneqq (1-16h^2/(\sqrt3\,d^2))^{-2}$.  Then
\[
 \varrho_h\le\eta_h\delta_h\,\frac{97\pi^4\nu^2}{d^4}.
\]
If $n_e\ge8$, then $\eta_h\delta_h<3/2$ and
$\varrho_h\le\bar\varrho \coloneqq 291\pi^4\nu^2/(2d^4)$.
\end{lemma}

\begin{proof}
We bound $\varrho_h$ by the Rayleigh quotient of an explicit test vector.
Let $\Phi(t) \coloneqq \sin^2(2\pi t/d)$ for
$0\le t\le d/2$ and $\Phi(t) \coloneqq 0$ for $-d/2\le t<0$.  Then
$\Phi(\pm d/2)=0$, the derivative $\Phi'(t)=(2\pi/d)\sin(4\pi t/d)$ on
$(0,d/2)$ is continuous at $0$ with $\Phi'(0)=0$, and
$\Phi''=(8\pi^2/d^2)\cos(4\pi t/d)$ on $(0,d/2)$.  Hence
\[
 \Phi\in W^{2,\infty}(-d/2,d/2)\subset H^2(-d/2,d/2),
\]
and
\[
 \|\Phi\|^2=\frac{3d}{16},\qquad\|\Phi'\|^2=\frac{\pi^2}{d},\qquad
 \|\Phi''\|^2=\frac{16\pi^4}{d^3},\qquad
 \frac{h^2}{\pi^2}\,\frac{\|\Phi''\|}{\|\Phi\|}=\frac{16h^2}{\sqrt3\,d^2}<1,
\]
where the last inequality holds because $n_e\ge4$.

Let $\hat a \coloneqq (\Phi(t_i))_i$, let $\hat b$ be
as in Lemma~\ref{lem:wm-oned}(d), and let $g \coloneqq \hat b\otimes\hat a$, so that
$g_r=\Phi(x_{r,1})\cos(\pi x_{r,2}/d)$.  Then $\hat a_i=0$ whenever
$t_i\le0$, so $\Pi_+g=g$.  By Lemma~\ref{lem:wm-oned}(c) and the last relation in the display above,
\[
 \|I^1_h\Phi\|\ge\|\Phi\|-\frac{h^2}{\pi^2}\|\Phi''\|
 =\Bigl(1-\frac{16h^2}{\sqrt3\,d^2}\Bigr)\|\Phi\|>0,
\]
so $\hat a\ne0$, and $\hat b>0$ entrywise.  Hence $g\ne0$ is
admissible in \eqref{eq:wm-varrho}.

With $M_D=M_1\otimes M_1$,
$K_0=\nu(M_1\otimes S_1+S_1\otimes M_1)$ and $S_1\hat b=\varpi_hM_1\hat b$
we get $K_0g=\nu(M_1\hat b)\otimes(S_1\hat a+\varpi_hM_1\hat a)$, and hence
\[
 \frac{g^\top K_0M_D^{-1}K_0g}{g^\top M_Dg}
 =\nu^2\,\frac{\hat a^\top S_1M_1^{-1}S_1\hat a+2\varpi_h\,\hat a^\top S_1\hat a
 +\varpi_h^2\,\hat a^\top M_1\hat a}{\hat a^\top M_1\hat a}.
\]

The lower bound for $\|I^1_h\Phi\|$ gives $\|I^1_h\Phi\|^{-2}\le\delta_h
\|\Phi\|^{-2}$, and $1\le\eta_h\le\delta_h$, since
$16/\sqrt3>\pi^2/6$ implies $\delta_h\ge\delta_h^{1/2}\ge\eta_h$.  Inserting
Lemma~\ref{lem:wm-oned}(a),(b),(d) into the Rayleigh quotient, we obtain
\begin{align*}
 \varrho_h&\le\nu^2\Bigl[\delta_h\,
 \frac{\|\Phi''\|^2+2\eta_h(\pi/d)^2\|\Phi'\|^2}{\|\Phi\|^2}
 +\eta_h^2\,\frac{\pi^4}{d^4}\Bigr]\\
 &\le\eta_h\delta_h\,\nu^2\Bigl[
 \frac{\|\Phi''\|^2+2(\pi/d)^2\|\Phi'\|^2}{\|\Phi\|^2}
 +\frac{\pi^4}{d^4}\Bigr]
 =\eta_h\delta_h\,\frac{97\pi^4\nu^2}{d^4},
\end{align*}
where the last equality uses the norms of $\Phi$ computed above: the
bracket equals
$(256+32+3)\pi^4/(3d^4)$.

Finally, if $n_e\ge8$, then $h^2/d^2\le1/64$,
so $\eta_h\le(1-\pi^2/384)^{-1}<1.0264$ and
$\delta_h\le(1-1/(4\sqrt3))^{-2}<1.3659$.  Hence
$\eta_h\delta_h<1.402<3/2$ and
$\varrho_h<(3/2)\cdot97\pi^4\nu^2/d^4=\bar\varrho$.
\end{proof}

The third theorem shows that, on the model problem, the order
$\gamma^{-1}$ in \eqref{eq:wm-scalar-kappa} cannot be removed by any
preconditioner that takes the same value at the two mirror masks.

\begin{theorem}[Obstruction and sharpness]\label{thm:wm-obstr}
Let Assumption~\ref{ass:wm-local} hold on the square $(-d/2,d/2)^2$ with
$n_e\ge3$ elements per direction and $a_{0,Tq}\equiv\nu>0$, assume
\eqref{eq:wm-exactquad}, let $\gamma>0$, and let $D^\pm$ be as defined
before \eqref{eq:wm-varrho} and $\varrho_h$ as in \eqref{eq:wm-varrho}.
\begin{enumerate}[label=\textup{(\roman*)},leftmargin=*]
\item For every SPD $Q\in\R^{N\times N}$,
 \begin{equation}\label{eq:wm-obstruction}
  \begin{gathered}
  \max_\pm\kappa_{\rm sp}\bigl(Q^{-1}P_W(D^\pm)\bigr)
  \ge1+\frac{1}{\gamma\varrho_h},\\
  \max_\pm\kappa_{\rm sp}\bigl(Q^{-1}J(D^\pm)\bigr)
  \ge1+\frac{1}{\gamma C_H\varrho_h}
  \ge\frac{\theta_-}{\theta_+}\Bigl(1+\frac{1}{\gamma\varrho_h}\Bigr),
  \end{gathered}
 \end{equation}
 where the second line assumes $c_HH_0\preceq H\preceq C_HH_0$ for
 constants $0<c_H\le C_H$ and $\theta_\pm$ are as in
 Theorem~\ref{thm:wm-equiv}(c).  For $Q=P_\vartheta$ with
 $\vartheta\ge0$, the first bound holds for each of the two masks.
\item If $n_e\ge8$, that is, $h\le d/8$, then
 $\varrho_h\le\bar\varrho=291\pi^4\nu^2/(2d^4)$.
\item Let $n_e\ge8$, take $\underline\lambda \coloneqq 2\pi^2\nu/d^2$ in
 \eqref{eq:wm-epsgamma}, so that
 $\varepsilon_\gamma=d^4/(4\pi^4\nu^2\gamma)$, and let
 $\vartheta\in[0,1]$ be fixed or any function of $D$ with values in
 $[0,1]$, such as $\operatorname{Tr}D/m$.  Then for every $\gamma>0$, we have
 \begin{equation}\label{eq:wm-twosided}
  1+\frac{8}{291}\,\varepsilon_\gamma
  \le\sup_{D}\kappa_{\rm sp}\bigl(P_\vartheta^{-1}P_W(D)\bigr)
  \le9\,(1+\varepsilon_\gamma),
 \end{equation}
 where the supremum is over diagonal $0\le D\le I_m$.  The lower bound
 already holds for $D=D^+$ and for $D=D^-$.
\item If $\psi_1\equiv1$, as for the orthonormal total-degree Legendre
 basis of Section~\ref{sec:numerics} with the zero multi-index listed first,
 then for every $\gamma>0$ there are
 $p^\pm\in\R^N$ and $\delta^\pm>0$ such that $D(p)=D^\pm$ whenever
 $\|p-p^\pm\|_2<\delta^\pm$, and targets $Y_d^\pm\in\R^N$ such that $p^\pm$
 is the unique solution of \eqref{eq:F} with $Y_d=Y_d^\pm$.
\end{enumerate}
\end{theorem}

\begin{proof}
(i) Let $P_\pm \coloneqq P_W(D^\pm)$.  We first show that
$\kappa_{\rm sp}(P_-^{-1}P_+)\ge\omega_\gamma^2$, that is, that $P_+$ and
$P_-$ are far apart.
Lemma~\ref{lem:wm-hilbert} then shows that no $Q$ is close to both.  By
Lemma~\ref{lem:wm-mirror}(c) and
Lemma~\ref{lem:wm-pencil}(a), test vectors in $\mathcal V_+$ give
$\lambda_{\max}(P_-^{-1}P_+)\ge\omega_\gamma$, and test vectors in
$\mathcal V_-$ give $\lambda_{\min}(P_-^{-1}P_+)\le\omega_\gamma^{-1}$.
Hence $\kappa_{\rm sp}(P_-^{-1}P_+)\ge\omega_\gamma^2$.
Lemma~\ref{lem:wm-hilbert} with $(A,B)=(P_-,P_+)$ gives
\[
 \omega_\gamma^2\le\kappa_{\rm sp}(Q^{-1}P_-)\,\kappa_{\rm sp}(Q^{-1}P_+)
 \le\Bigl(\max_\pm\kappa_{\rm sp}(Q^{-1}P_\pm)\Bigr)^2,
\]
and taking square roots gives the first bound in
\eqref{eq:wm-obstruction}.  The same argument
with $J(D^\pm)$ and $\omega_\gamma^J$ gives the first inequality for $J$.
For the second inequality, if $C_H\ge1$, then
$\theta_+=C_H$ and $\theta_-\le1$, so
\[
 \frac{\theta_-}{\theta_+}\,\omega_\gamma\le\frac{\omega_\gamma}{C_H}
 =\frac1{C_H}+\frac{1}{\gamma C_H\varrho_h}\le\omega_\gamma^J .
\]
If $C_H<1$, then $\theta_+=1$ and $\theta_-=c_H\le C_H$, so
$\theta_-\omega_\gamma\le C_H+C_H(\gamma\varrho_h)^{-1}
\le1+(\gamma C_H\varrho_h)^{-1}=\omega_\gamma^J$.  Finally, for
$Q=P_\vartheta$, Lemma~\ref{lem:wm-mirror}(b) gives
$P_\vartheta^{-1}P_-=\widetilde{\mathsf F}(P_\vartheta^{-1}P_+)
\widetilde{\mathsf F}^\top$.  Thus $P_\vartheta^{-1}P_+$ and
$P_\vartheta^{-1}P_-$ are similar, so their condition numbers coincide and
each equals the maximum in the first bound of \eqref{eq:wm-obstruction}.

(ii) This is Lemma~\ref{lem:wm-rho}.

(iii) By (ii) and $\underline\lambda=2\pi^2\nu/d^2$,
\[
 \frac{1}{\gamma\varrho_h}\ge\frac{1}{\gamma\bar\varrho}
 =\frac{\underline\lambda^2}{\bar\varrho}\,\varepsilon_\gamma
 =\frac{4\pi^4\nu^2/d^4}{291\pi^4\nu^2/(2d^4)}\,\varepsilon_\gamma
 =\frac{8}{291}\,\varepsilon_\gamma .
\]
Let $D$ be one of the masks $D^+$ and $D^-$, and let
$\vartheta' \coloneqq \vartheta(D)$.  The last statement of part (i), with
$Q=P_{\vartheta'}$, gives
$\kappa_{\rm sp}(P_{\vartheta'}^{-1}P_W(D))\ge1+(8/291)\varepsilon_\gamma$,
which is the lower bound in \eqref{eq:wm-twosided}.  For the upper bound,
$\Lambda_L=9$ and $\underline\lambda=2\pi^2\nu/d^2$ are admissible in
\eqref{eq:wm-lump} by Lemmas~\ref{lem:wm-lump}(b) and~\ref{lem:wm-weyl}(a),
since $\nu_-=\nu$.  Theorem~\ref{thm:wm-equiv}(b) therefore gives
$\kappa_{\rm sp}(P_\vartheta^{-1}P_W(D))\le\chi_\gamma(\vartheta)
\le9(1+\varepsilon_\gamma)$ for every diagonal $0\le D\le I_m$
and every $\vartheta\in[0,1]$.

(iv) %\emph{Step 1 (the points $p^\pm$).} 
Let $\psi_1\equiv1$, let
$e_1\in\R^{n_\xi}$ be the first unit vector, and recall that $a<b$ are the
bounds of the control box.  Define $u_{\rm f} \coloneqq (a+b)/2$, $u_{\rm s} \coloneqq b+1$
and $p^\pm \coloneqq e_1\otimes z^\pm$, where $z^\pm\in\R^{n_h}$ has the entries
$z^\pm_r \coloneqq \gamma u_{\rm f}$ if $x_r\in\mathcal O_\pm$ and
$z^\pm_r \coloneqq \gamma u_{\rm s}$ otherwise.  Then
$(Ep^\pm)_{(k,r)}=\psi_1(\xi_k)z^\pm_r=z^\pm_r$, so $(Ep^\pm)_{(k,r)}/\gamma$
lies in $(a,b)$ exactly when $x_r\in\mathcal O_\pm$ and equals
$u_{\rm s}\notin[a,b]$ otherwise.  Thus $D(p^\pm)=D^\pm$.

%\emph{Step 2 (stability of the mask).} 
Let $\delta \coloneqq \min\{(b-a)/2,1\}$
and $\delta^\pm \coloneqq \gamma\delta/\|E\|_2$.  Every $p$ with
$\|p-p^\pm\|_2<\delta^\pm$ satisfies
\[
 \bigl|(Ep)_q-(Ep^\pm)_q\bigr|/\gamma\le\|E\|_2\,\|p-p^\pm\|_2/\gamma<\delta
 \qquad\text{for all }q .
\]
Hence the components of $Ep/\gamma$ at which $D^\pm$ is free stay in
$(u_{\rm f}-\delta,u_{\rm f}+\delta)\subset(a,b)$, and the others stay in
$(u_{\rm s}-\delta,u_{\rm s}+\delta)\subset(b,\infty)$, so that
$D(p)=D^\pm$.

Finally, define
\[
 Y_d^\pm \coloneqq \mathcal K^{-1}\bigl(\mathcal K\mathcal M^{-1}\mathcal K^\top p^\pm
 +E^\top W\Proj_{[a,b]}(Ep^\pm/\gamma)\bigr).
\]
Then $F(p^\pm)=0$ in \eqref{eq:F} with $Y_d=Y_d^\pm$.  The function $-F$
is the gradient of the dual objective in \eqref{eq:discrete-dual}, which is
strongly concave by the proof of Theorem~\ref{thm:discrete-dual}.  Hence
$p^\pm$ is its unique maximizer and the unique solution of \eqref{eq:F}.
\end{proof}
